# Supplementary material for: Covertly Controlling a Linear System
Source: arXiv:2212.01052 source file (2022-12-02)
Supplement: Supplementary file 1 [file additional_literature.tex]

% מאמרים נוספים הנוגעים לאבטחה בבקרה

% על איזו בעיה מדובר
% מה הם הראו
% איך זה שונה מהעבודה שלנו

% מאמרים שאסף שלח
C. Fang, Y. Qi, J. Chen, R. Tan and W. X. Zheng, "Stealthy Actuator Signal Attacks in Stochastic Control Systems: Performance and Limitations," in IEEE Transactions on Automatic Control, vol. 65, no. 9, pp. 3927-3934, Sept. 2020, doi: 10.1109/TAC.2019.2950072.

Investigated the trade-off between the attack detectability and the performance degradation in stochastic cyber-physical systems. 
The authors considered a linear time-invariant system in which the attack detector performs a hypothesis test on the innovation of the Kalman filter to detect malicious tampering with the actuator signals. 
% Similar to...
% but extending to (epsilon, delta)-stealthiness
They adopt a notion of attack stealthiness to quantify the degree of stealth by limiting the maximum achievable exponents of both false alarm probability and detection probability below certain thresholds. 
% And the conditions for any actuator attack to have a specific level of stealthiness are derived. 
% Additionally, we characterize the upper bound of the
% performance degradation induced by attacks with a given extent of
% stealthiness that produces independent and identically distributed
% Gaussian innovations, and design the attack, which achieves the
% stated upper bound for right-invertible systems. 
% Finally, our results
% are illustrated via numerical examples

L. An and G. -H. Yang, "Data-Driven Coordinated Attack Policy Design Based on Adaptive  $\mathcal{L}_2$-Gain Optimal Theory," in IEEE Transactions on Automatic Control, vol. 63, no. 6, pp. 1850-1857, June 2018, doi: 10.1109/TAC.2017.2753466.

Investigates from the attacker’s
standpoint, how an adversary should design a sensor–actuator coordinated attack policy to degrade a LTI system performance while staying undetected, without exact knowledge of the system matrices.
To guarantee that the attacker is undetected, the authors introduced the notion of $\alpha$-probability $\mathcal{L}_2$ stealthiness. 
They measure the attack’s impacts while ensuring the stealth capabilities
using $\mathcal{L}_2$-gain. 
% As a result, the attack goal is formulated as a data-based $\mathcal{L}_2$-gain composite optimization problem. Under this framework, a new multi-objective adaptive dynamic programming (ADP) method is proposed for
% launching the attack policy, which extends the traditional single-objective ADP technique. A numerical example is presented to
% demonstrate the effectiveness of the proposed attack scenarios.

D. Mikhaylenko and P. Zhang, "Stealthy Local Covert Attacks on Cyber-Physical Systems," in IEEE Transactions on Automatic Control, doi: 10.1109/TAC.2021.3131985.

Introduces a new attack strategy called a local covert
attack. 
This attack does not require access to all control input signals and sensor output signals, so it needs fewer disruption resources. 
They showed that the local covert attack can be made completely stealthy by applying the decoupling technique or by combining the basic idea of a covert attack and a zero-dynamics attack.

A. Barboni, H. Rezaee, F. Boem and T. Parisini, "Detection of Covert Cyber-Attacks in Interconnected Systems: A Distributed Model-Based Approach," in IEEE Transactions on Automatic Control, vol. 65, no. 9, pp. 3728-3741, Sept. 2020, doi: 10.1109/TAC.2020.2998765.

Distributed detection of covert attacks for linear large-scale interconnected systems is addressed in this
article.
This article focuses on large-scale systems subject to bounded process and measurement disturbances, where a single subsystem is under a covert attack. 
Here each subsystem can detect the presence of covert attacks in neighboring subsystems in a distributed manner. 
The detection strategy is based on the design of two model-based observers for each subsystem using only local information.

% מאמרים של הבודקים

b.	"Learning-based attacks in cyber-physical systems." IEEE Transactions on Control of Network Systems 8, no. 1 (2020): 437-449.

Introduces the problem of learning-based
attacks in a CPS for the case of a discrete-time, LTI system that
may be subject to an attack that overrides sensor readings
and controller actions. 
% The attacker attempts to learn the
% dynamics of the plant and subsequently overrides the controller’s actuation signal to destroy the plant without being
% detected. 
% The attacker can feed fictitious sensor readings
% to the controller using its estimate of the plant dynamics
% and mimic the legitimate plant operation. 
The controller, in
contrast, is constantly on the lookout for an attack; once
the controller detects an attack, it immediately shuts the
plant off. 
In the case of scalar plants, we derive an upper bound on the attacker’s deception probability for any measurable control policy when the attacker uses an arbitrary learning algorithm to estimate the system dynamics.
We then derive lower bounds for the attacker’s deception
probability for both scalar and vector plants by assuming
an authentication test that inspects the empirical variance
of the system disturbance. 
We also show how the controller can improve the security of the system by superimposing a carefully crafted privacy-enhancing signal on top of the
“nominal control policy.” 
% Finally, for nonlinear scalar dynamics that belong to the reproducing kernel Hilbert space, we investigate the performance of attacks based on nonlinear Gaussian process learning algorithms.

"Observability of Discrete-Time LTI Systems Under Unknown Piece-Wise Constant Inputs." IEEE Control Systems Letters 5, no. 6 (2020): 1886-1891

Deals with the observability of discrete-time LTI systems under unknown piece-wise constant inputs with sufficiently slow, but arbitrary update times. 
Under the assumption of knowing the update times, the authors characterized the unobservable subspace and showed that with sufficiently many measurements in each inter-update interval of the input, the unobservable subspace remains fixed. 
% They also explored the implications of the result for privacy in event-triggered control through an illustrative example.

"The value of timing information in event-triggered control." IEEE Transactions on Automatic Control 65, no. 3 (2019): 925-940

Studied event-triggered control for stabilization of unstable linear plants over rate-limited communication channels subject to unknown bounded delay. 
The authors showed that a phase transition behavior in the transmission
rate required for stabilization using a given event-triggering
strategy in order to compensate on the implicit information about the state of the plant, and the information loss causes by the delay in the communication channel.

% On one hand, the timing of event triggering carries
% implicit information about the state of the plant. On the
% other hand, the delay in the communication channel causes
% information loss, as it makes the state information available
% at the controller out of date. Combining these two effects,
% we show a phase transition behavior in the transmission
% rate required for stabilization using a given event-triggering
% strategy. 
% For small values of the delay, the timing information carried by the triggering events is substantial, and the system can be stabilized with any positive rate. 
% When the delay exceeds a critical threshold, the timing information alone is not enough to achieve stabilization, and the required rate grows. 
% When the delay equals the inverse of the entropy rate of the plant, the implicit information carried by the triggering events perfectly compensates the loss of information due to the communication delay, and we recover the rate requirement prescribed by the data-rate theorem. 
% We also provide an explicit construction yielding a sufficient rate for stabilization, as well as results for vector systems. 
% Our results do not rely on any a priori probabilistic model for the delay or the initial conditions.

Mo and Sinopoli entitled "False data injection attacks in control systems"

This paper analyzes the effects of false data injection attacks on Control System. 
Assuming that the system equipped with a Kalman filter, failure detector, and LQG controller is used to monitor and control a discrete LTI Gaussian system. 
% We further assume that the system is equipped with a failure detector.
An attacker wishes to destabilize the system by compromising
a subset of sensors and sending corrupted readings to
the state estimator. 
In order to inject fake sensor measurements without being detected the attacker needs to carefully design its inputs to fool the failure detector.
% since abnormal sensor measurements usually trigger an alarm from the failure detector. 
The authors provided a necessary and sufficient condition under which the attacker could destabilize the system while successfully bypassing the failure detector. 
A design method for the defender to improve the resilience of the CPS against such kind of false data injection attacks is also provided.
